# Supplementary material for: Social interaction, noise and antibiotic-mediated switches in the intestinal microbiota
Source: arXiv:1203.2883 source file (2012-03-13)
Supplement: Supplementary file 1 [file SupplementaryMaterialNew2.pdf]

## Social interaction, noise and antibiotic-mediated switches in the intestinal microbiota

Vanni Bucci, Serena Bradde, and Joao B. Xavier
*Program in Computational Biology, Memorial Sloan-Kettering Cancer Center, New York, U.S.A.*

Giulio Biroli
*Institut Physique Théorique (IPhT) CEA Saclay,*
*and CNRS URA 2306, 91191 Gif Sur Yvette, France*

### I. MODEL AND STABILITY ANALYSIS

#### A. Four-dimensional model

We determine the expressions of four biologically meaningful rest points by setting to zero the right-hand sides (rhs) of eqs. 6 in the main text. The first trivial fixed point $\mathbf{P}_0 = (1, 0, 0, 1)$ is the one where both bacterial groups are extinct. The second fixed point $\mathbf{P}_1 = (\mu_s, (1 - \mu_s)/\epsilon, 0, 1)$ represents the sensitive monoculture where $\mu_s = -(a\epsilon)/(\epsilon - m_s)$, and $\mu_t = a/(m_t - 1)$. $\mu_s$ and $\mu_t$ are the chemostat parameters reflecting the break-even concentrations of $\rho_s$ and $\rho_t$ without antibiotic presence [1].

This point has to be positive-definite thus identifying the following conditions: i) $m_s > \epsilon$ and ii) $m_s > \alpha\epsilon$. The third fixed point $\mathbf{P}_2 = (\mu_t, 0, 1 - \mu_t, 1)$ represents the scenario of tolerants monoculture. This point exists given the necessary conditions: i) $m_t > 1$ and ii) $m_t > \alpha$. The last rest point, $\mathbf{P}_3 = (\mu_s, \rho_{s_3}, \rho_{t_3}, 1)$ corresponds to the scenario of coexistence where the expression for the bacterial concentrations are respectively:

$$\rho_{s_3} = \frac{1}{\psi}\left(\frac{m_t}{m_s}\,\epsilon - 1\right)$$
$$\rho_{t_3} = \frac{m_s}{m_t}\left(\frac{a}{\epsilon - m_s} + \frac{1}{\psi} + \frac{1}{\epsilon}\right) - \frac{\epsilon}{\psi}\,. \tag{1}$$

Three conditions are necessary for the positivity of $\boldsymbol{\rho}_3$: i) $m_s > \epsilon$, ii) $\epsilon\, m_t > m_s$ and iii) $\psi < \frac{\epsilon(\epsilon - m_s)(\epsilon m_t - m_s)}{m_s(\epsilon\alpha - m_s)}$. Since the parameters are positive, condition iii) gives the additional constrain of $m_s > \epsilon\alpha$.

The stability of the system is studied by linearising equations reported in 6 of the main text around each rest point and computing the eigenvalues of the relative Jacobian matrix, defined by:

$$\mathbf{J} = \begin{bmatrix} -\frac{a(m_s\rho_s + m_t\rho_t)}{(a+S)^2} - 1 & -\frac{m_s}{a+S}S & -\frac{m_t}{a+S}S & 0 \\ \frac{am_s}{(a+S)^2}\rho_s & \frac{m_s}{a+S}S - \epsilon & 0 & 0 \\ \frac{am_t}{(a+S)^2}\rho_s & -\psi\rho_t & \frac{m_t}{(a+S)}S - \psi\rho_s - 1 & 0 \\ 0 & 0 & 0 & -1 \end{bmatrix} \tag{2}$$

The eigenvalues relative to $\mathbf{J}_{\mathbf{P}_0}$ are $\lambda_1^0 = -1, \lambda_2^0 = -1, \lambda_3^0 = -\frac{m_t}{a+1} - 1, \lambda_4^0 = -\frac{m_s}{a+1} - \epsilon$. $\mathbf{P}_0$ is stable if all eigenvalues $\boldsymbol{\lambda}^0$ are negative, which determines the following inequalities: i) $m_t < \alpha$ and ii) $m_s < \alpha\epsilon$. It is worth noticing that the conditions ensuring the stability of $\mathbf{P}_0$ are the opposite of those for the existence of $\mathbf{P}_1$ and $\mathbf{P}_2$.

Similarly, the stability for $\mathbf{P}_1$ are determined by studying the sign of the following eigenvalues: $\lambda_1^1 = -1, \lambda_2^1 = \frac{\psi(\mu_s - 1)}{\epsilon} + \frac{\mu_s m_t}{a + \mu_s} - 1, \lambda_{3,4}^1 = -\sigma \pm \sqrt{\sigma^2 - \frac{4\epsilon a^3 m_s^3(\epsilon(a+1) - m_s)}{(\epsilon - m_s)^3}}$, where $\sigma = \frac{am_s[am_s + (\epsilon(a+1) - m_s)(\epsilon - m_s)]}{2(a+\mu_s)^2(\epsilon - m_s)^2}$. Imposing $\lambda_2^1 < 0$ gives the following inequalities: i) $m_s > \epsilon$ and ii) $m_s/m_t > \frac{\epsilon^2}{\psi(1-\mu_s) + \epsilon}$. The conditions for $\lambda_{3,4}^1 < 0$ are equivalent to those for $\mathbf{P}_1$ existence. In summary, if $\mathbf{P}_1$ is well-defined, it is stable given the condition ii).

The eigenvalues associated to $\mathbf{J}_{\mathbf{P}_2}$ read: $\lambda_1^2 = -1, \lambda_2^2 = -1, \lambda_3^2 = m_s/m_t - \epsilon, \lambda_4^2 = -\frac{(m_t - 1)^2 - a(m_t - 1)}{am_t}$. The conditions for local stability of $\mathbf{P}_2$ are: i) $m_t > \alpha$ and ii) $m_s/m_t < \epsilon$.

To study the stability of $\mathbf{P}_3$, we used the Routh-Hurwitz criteria [4]. Let $p = r^4 + c_1 r^3 + c_2 r^2 + c_3 r + c_4$ being the fourth-order characteristic polynomial for $\mathbf{J}_{\mathbf{P}_3}$, then the rest point $\mathbf{P}_3$ is stable given the necessary and sufficient conditions: i) $c_1 > 0$, ii) $c_3 > 0$, iii) $c_4 > 0$ and iv) $c_1 c_2 c_3 > c_3^2 + c_1^2 c_4$. It is easy to verify that conditions i) and ii) are always satisfied:

$$c_1 = \frac{(\epsilon + m_s)}{m_s} + \frac{(\epsilon - m_s)^2}{m_s} > 0$$

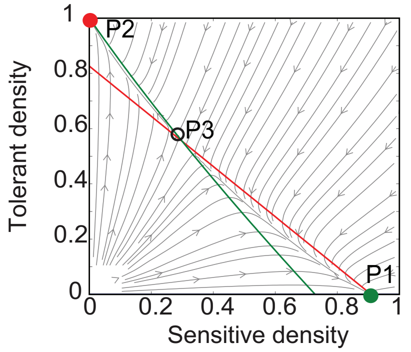


FIG. S1: In figure we present the vectorial field of forces and the phase-plane analysis for bistable conditions, for the following parameter values: ratio between tolerant and sensitive maximum growth rate $f = 1.1$, antibiotic killing rate $\epsilon = 1.1$ and social interaction rate $\psi = 0.7$. We draw the three rest points $\boldsymbol{\rho}_1$ (blue circle), $\boldsymbol{\rho}_2$ (red circle) and $\boldsymbol{\rho}_3$ (empty circle), where $\boldsymbol{\rho} = (\rho_s, \rho_t)$ is the vector having for components the sensitive $s$ and tolerant $t$ densities, and the system nullclines defined by $d\rho_s/dt = 0$ (red line), $d\rho_t/dt = 0$ (blue line) whose intersection individuate the saddle unstable rest point $\boldsymbol{\rho}_3$.

$$c_3 = \frac{a}{(a+\mu_s)^3}[m_s\rho_{c_3} + m_t\rho_{p_3} + m_s m_t \psi \rho_{c_3}\rho_{p_3}] > 0$$

However, it is also fairly easy to see that condition iii) does not hold. Given the expression for $c_4$

$$c_4 = \frac{\epsilon\rho_{c_3}(\epsilon - m_s)^2[m_s(1+\psi\rho_{c_3}) - m_t(\epsilon + \psi\rho_{p_3})]}{a m_s^2},$$

condition iii) requires that $m_s(1+\psi\rho_{c_3}) > m_t(\epsilon + \psi\rho_{p_3})$. After some algebra we can see that this condition is false when the rest point is well-defined.

It is now possible to determine the criteria describing the system mono- or bistability in function of the model parameters. By assuming the existence of both fixed points and by comparing the conditions of stability obtained from the linearisation analysis we derive the following relationships:

- Monostability with only sensitives $\frac{m_t}{m_s}\epsilon < 1$
- Monostability with only tolerants $\frac{m_t}{m_s}\epsilon > 1 + \frac{\psi}{\epsilon}(1-\mu_s)$
- Bistability with both mutually exclusive sensitives and tolerants monocultures $1 < \frac{m_t\epsilon}{m_s} < 1 + \frac{\psi}{\epsilon}(1-\mu_s)$

These criteria highlight two major concepts. First, there is necessity for a negative feedback (i.e. $\psi > 0$) from sensitives to tolerants for bistability to arise. If no negative feedback is present the system can set only in one of the two mono-stable states. Second, the modulation effect of the antibiotic $\epsilon$. It is clear that an increase in antibiotic-killing action needs to be counteracted by an increase in selective pressure in order to maintain proper balance.

### B. Two-dimensional model

The two dimensional model of eqs. (1) and (2) in the main text is obtained by: 1) substituting eq. (7) of the main text into eq. (6), 2) simplifying the saturation terms by dividing numerator and denominator by $m_s$ and 3) introducing $f = m_t/m_s$.

We repeat the linear stability analysis finding three equivalent fixed points (Fig. S1): $\boldsymbol{\rho}_1 = (1/\epsilon, 0)$, which represents the sensitive monoculture, $\boldsymbol{\rho}_2 = (0, 1)$, which represents the tolerants monoculture and $\boldsymbol{\rho}_3 = (\frac{\epsilon f - 1}{\psi}, \frac{\psi + \epsilon(1-\epsilon f)}{\psi \epsilon f})$ which represents a state where both groups coexist. States 1 and 2 are always well-defined while state 3 exists if and only if $1 < \epsilon f < 1 + \psi/\epsilon$. The Jacobian matrix $\mathbf{J}(\boldsymbol{\rho})$ now reads

$$\mathbf{J}(\boldsymbol{\rho}) = \begin{bmatrix} \frac{f\rho_t}{(\rho_s + f\rho_t)^2} - \epsilon & -\frac{f\rho_s}{(\rho_s + f\rho_t)^2} \\ -\psi\rho_t - \frac{f\rho_t}{(\rho_s + f\rho_t)^2} & \frac{f\rho_s}{(\rho_s + f\rho_t)^2} - \psi\rho_s - 1 \end{bmatrix} \quad (3)$$

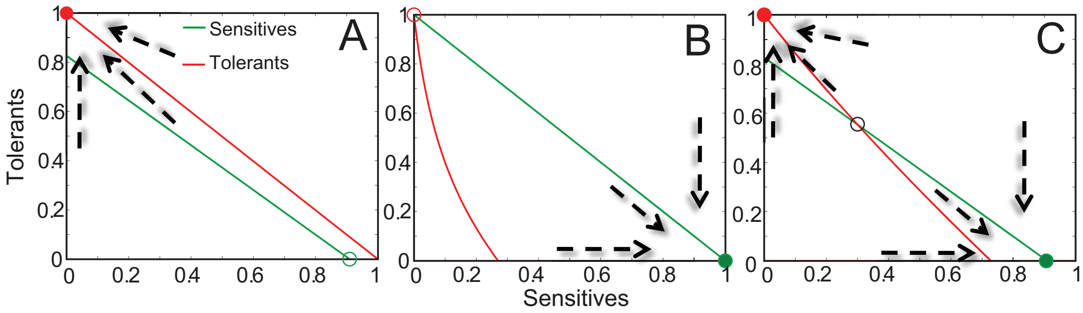


FIG. S2: Model nullclines analysis in the absence of noise. A the tolerants nullcline lies above the sensitives nullcline leading to tolerants dominance and sensitive extinction. The corresponding parameter set is $f = 1.1, \epsilon = 1.1, \psi = 0.1$. B the sensitives nullcline lies above the tolerants nullcline leading to sensitives dominance and tolerants extinction. The corresponding parameter set is $f = 1.0, \epsilon = 1.0, \psi = 5$. C The tolerants nullcline is steeper than the sensitives nullcline and their intersection is a saddle and unstable point. The stable manifold of the saddle divides the interior of the quadrant into the sets of initial conditions leading to competitive dominance by one type of microbe and competitive exclusion of the other. The corresponding parameter set is $f = 1.1, \epsilon = 1.0, \psi = 0.7$.

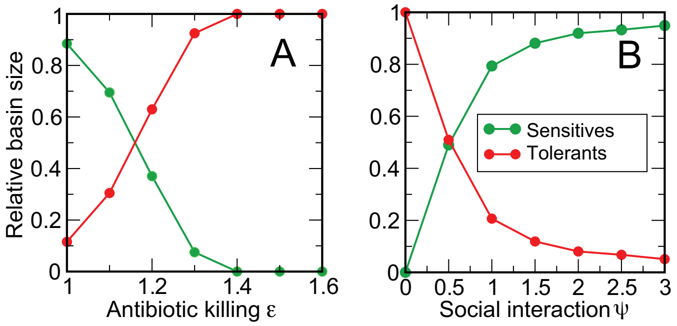


FIG. S3: Normalized-to-one areas of the basins of attraction, corresponding to sensitives (green curve) and tolerants (red curve), versus the antibiotic-killing $\epsilon$ or the social interaction $\psi$.

$\boldsymbol{\rho}_1$ has eigenvalues $\lambda_1 = -\epsilon$ and $\lambda_2 = \epsilon f - \psi/\epsilon - 1$. Thus, since $\epsilon$ is positive-defined, $\boldsymbol{\rho}_1$ is stable if and only if $\epsilon f < 1 + \psi/\epsilon$. Equivalently, eigenvalues in state 2 are $-1$ and $1/f - \epsilon$ meaning that it is stable if and only if $\epsilon f > 1$. Since the characteristic polynomial of $\mathbf{J}$ is $p = r^2 + c_1 r + c_2$ the conditions for $\boldsymbol{\rho}_3$ local stability are $c_1 = -\lambda_1 - \lambda_2 > 0$ and $c_2 = \lambda_1\lambda_2 > 0$. These conditions are equivalent to verifying that the real parts of $\lambda_1$ and $\lambda_2$ are strictly negative. The expression for $c_1$ and $c_2$ are the following:

$$c_1 = \epsilon f - \frac{\epsilon^2(1-f)(1-\epsilon f)}{\psi}$$

$$c_2 = \epsilon\frac{(1-\epsilon f)}{\psi}[\epsilon(1-\epsilon f) + \psi]$$

The first condition implies that $\psi/\epsilon > (1-\epsilon f)(1-f)/f$. The conditions is true only in the particular case when $f > 1$, which by itself does not prove the instability of state 3. However, in order to have $c_2 > 0$, the argument inside the square bracket has to be negative $\psi/\epsilon < \epsilon f - 1$ which is the opposite of the one ensuring $\boldsymbol{\rho}_3$ existence. As a consequence, if state 3 exists, it will be locally unstable as it is for the four dimensional model. We show that the simplification of steady state and complete consumption of the substrate does not alter the analysis of the model and we end finding the same qualitative phase diagram of the previous model.

The system stability features can be visualized by drawing the system nullclines (i.e. the curves represented by $\frac{d\rho_s}{dt} = 0$ and $\frac{d\rho_t}{dt} = 0$) in the phase-plane defined by tolerant $\rho_t$ vs. sensitive $\rho_s$ density (Fig. S2). Tolerants domination $\boldsymbol{\rho}_2$ is always obtained for parameter sets resulting in the tolerants nullcline laying above the sensitives one (Fig. S2A) and the reverse is true for sensitives dominance $\boldsymbol{\rho}_1$ (Fig. S2B). Bistability is obtained when the nullclines intersect in

the saddle unstable coexistence point $\boldsymbol{\rho}_3$ such that the stable manifold of the saddle divides the interior of the quadrant into the sets of initial conditions leading to competitive dominance by one type of microbe and competitive exclusion of the other. In absence of fluctuations, depending on the initial conditions a time-trajectory will be attracted in one of the two mutually exclusive stable states $\boldsymbol{\rho}_1$ or $\boldsymbol{\rho}_2$ depending on the initial condition and that long-term steady state will persist for ever (Fig. S2C).

The phase-plane is divided into two attracting basins, one around the tolerant mono-culture and the other around the sensitive mono-culture whose size was calculated with a Monte Carlo search in the phase space (Fig. S3).

## II. RANDOM FLUCTUATION AND NOISE-INDUCED DYNAMICS

The integration of the Langevin dynamics in presence of bistability shows that the system time evolution in presence of random exposure is non-trivial. The micriobiota switches over-time between the tolerant- and the sensitive-dominated states (and vice-versa) which was also observed experimentally [6]. Moreover, these switch times are not-deterministic and vary for different realizations of the random fluctuations. We first show how to characterize the location of long-term states and then describe in details the method used to compute the mean residence time both numerically and theoretically.

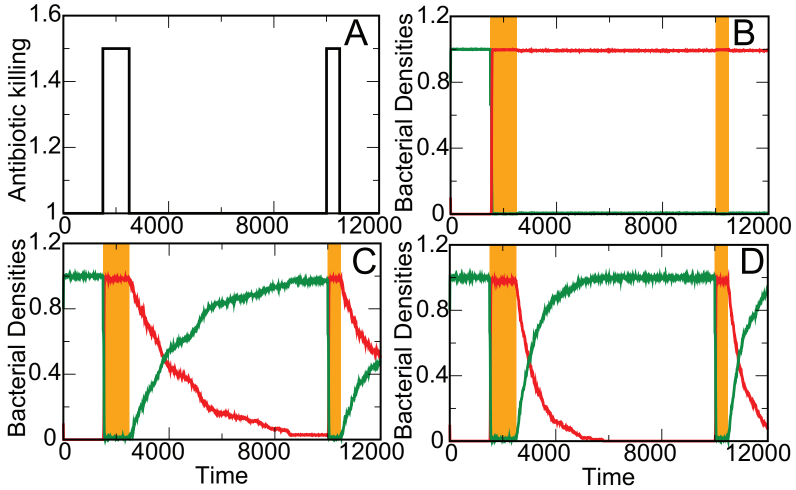


FIG. S4: Time evolution of the sensitive and tolerant concentrations obtained by solving the Langevin equations for $f = 1.1$, $\psi = 0.7$, $\epsilon$ variable with time (see Panel A) and three different noise regimes. A) antibiotic treatment B) $D \to 0$, C) $D = 0.00033$ and D) $D = 0.001$. The densities are obtained averaging over 100 noise realizations and show the strong dependence of the return to sensitive domination after treatment on the noise level. Orange shaded region represents treatment conditions. The dynamics here shown qualitatively reproduces the behaviour observed in longitudinal microbiome data (see Fig. 5).

Intuitively, we can think that the introduction of random exposure leads to diffusion within the space of possible configurations making therefore the time of escape from each stable or meta-stable state strictly finite due to the noise-activated dynamics. The strength of the diffusive motion is given by $D$. This suggests that by increasing the amplitude of the fluctuations $D$, the system needs a shorter time to wander far from the initial configuration therefore increasing the probability of crossing the separatrix in smaller time.

Previous studies have characterized the mean residence time computing the escape rate between the two stable states in the small $D$ limit in terms of the stationary probability distribution [8, 9]. However, in our case this function is not known a priori since the system is non-conservative. Alternative numerical solutions (explicit integration of the Langevin equations or of the Fokker-Planck Equation) can be used to do so. However, these methods can be very numerically intensive, and become prohibitive when the number of states increases (i.e. solving a partial differential equation in $d \gg 3$ dimensions). As a consequence, we followed a new alternative theoretical framework based on transition state theory.

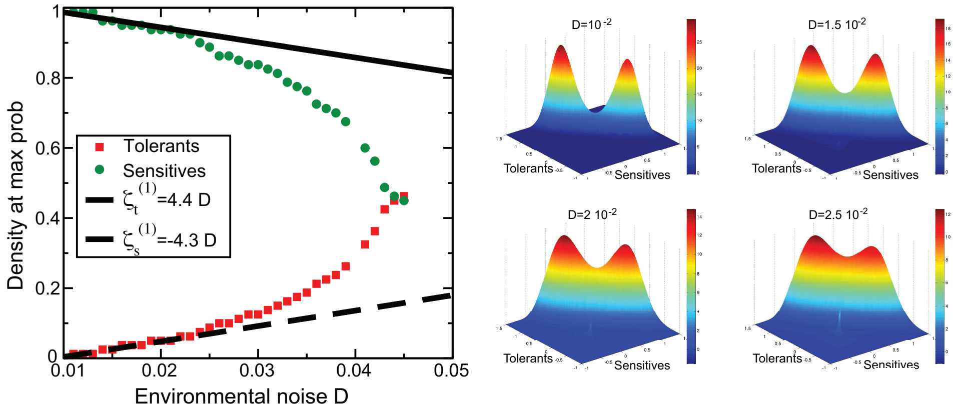


FIG. S5: In the left panel we show how the most probable concentration $\boldsymbol{\rho}$ changes with respect the noise parameter $D$ when the boundary condition are fixed at negative values far away from the location of stable points for the set of parameters $f = 1.1, \epsilon = 1.1$ and $\psi = 0.4$. This configuration is not physical since we allow negative values of the concentrations but we show the theoretical prediction of the linear coefficients perfectly matches the numerical data. In the right panel we show 4 different stationary distributions for $f = 1.1, \epsilon = 1.1, \psi = 0.4$ and $D = 0.01, 0.015, 0.02, 0.025$ obtained solving numerically the FPE with boundary conditions: $P^s(-1, \rho_t) = 0$ and $P^s(\rho_s, -1) = 0$.

### *Numerical estimates of the mean residence time*

In order to characterize the stochastic dynamical behaviour of the bacterial concentrations we can estimate numerically the moments of the joint probability distribution of bacterial concentration, $P(\boldsymbol{\rho})$, by sampling different possible trajectories connecting the two monoculture states multiple times. Each time-trajectory is obtained by solving the Langevin equations with different realizations of the noise $\boldsymbol{\xi}$ using a Milstein integration scheme [7]. We compare the sampled frequency of being in one of the two states to the stationary probability distribution obtained by solving the FP equation. Moreover this sampling technique allows us to compute the average time $t_i$ that the microbiota spends in each stable states computing the fraction of time the microbiota is located in one of the stable states $i = 1, 2$.

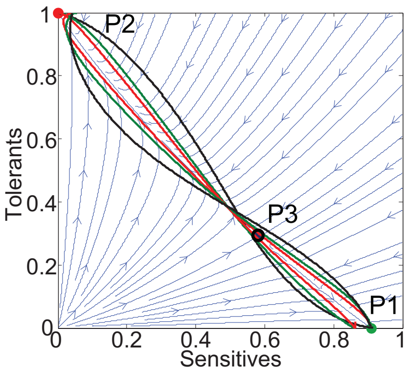


FIG. S6: The figure shows the stationary path connecting the stable points 1 and 2. The red, green and black solid curves are the trajectory associated with different values of the initial velocity, 0.032 0.072 and 0.172 respectively showing the most probable path for small noise is concentrated along the unstable manifold as obtained for different sampled trajectory (data not shown). It is worth emphasizing that for conservative fields of forces, meaning $\mathbf{F} = -\boldsymbol{\nabla} U$, it easy to verify that $\dot{\boldsymbol{\rho}} = \pm\mathbf{F}$ are both the uphill and downhill optimal path. The solution with the plus sign has null action $\mathcal{S} = 0$ meaning that its probability is equal to unity for every value of the noise $D$. This means that the path is always deterministic: it describes a simple gradient descent that takes place even in absence of noise. On the contrary the $\dot{\boldsymbol{\rho}} = -\mathbf{F}$ is associated to the reverse path and has a finite action $\mathcal{S} > 0$ meaning it is activated only in presence of noise since its probability is suppressed and has strictly null value when $D = 0$. The optimal path connecting two stable states is formed by an ascending trajectory toward the unstable point, given by $\dot{\boldsymbol{\rho}} = -\mathbf{F}$, followed by a descending trajectory given by $\dot{\boldsymbol{\rho}} = \mathbf{F}$. In presence of a non-conservative force, the scenario changes completely and the uphill and downhill trajectory are different since $\dot{\boldsymbol{\rho}} = -\mathbf{F}$ is not a solution of the optimal path equation any longer.

## III. SUPPORTING FIGURES FOR SVD

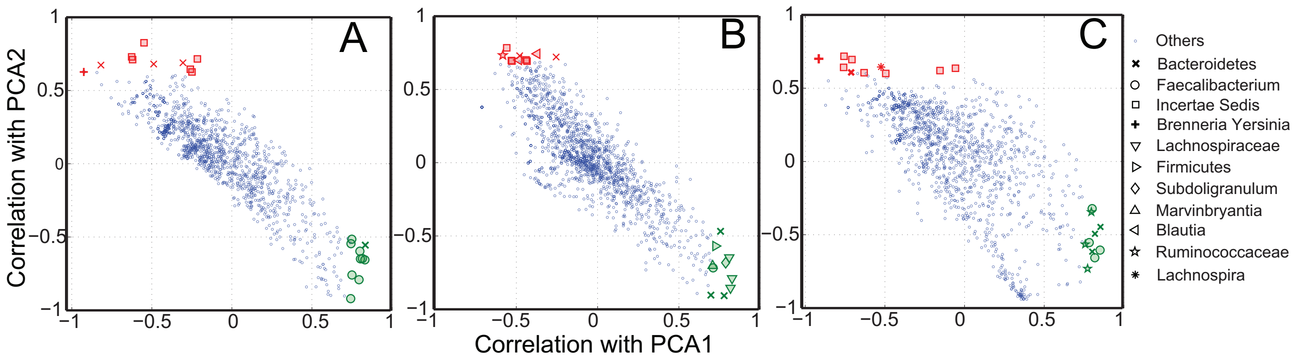


FIG. S7: Plot of the correlation with principal component 2 (PCA2) versus correlation with principal component 1 (PCA1) for all the phylotypes detected in each individual (A,B,C) from [2]. Green (red) are the top 10 most correlated phylotypes with PCA1 (PCA2) which significantly decrease (increase) in response to antibiotic treatment. Confirming what observed in [2] phylotypes of the genus *Faecalibacterium* and *Lachnospiraceae* are indicative of unperturbed samples and form the sensitive class. Similarly it appears that the *Incertae sedis* genus characterizes the tolerant class. Interestingly genus such as *Bacteroidetes* and *Ruminococcaceae* have representative phylotypes in both classes.

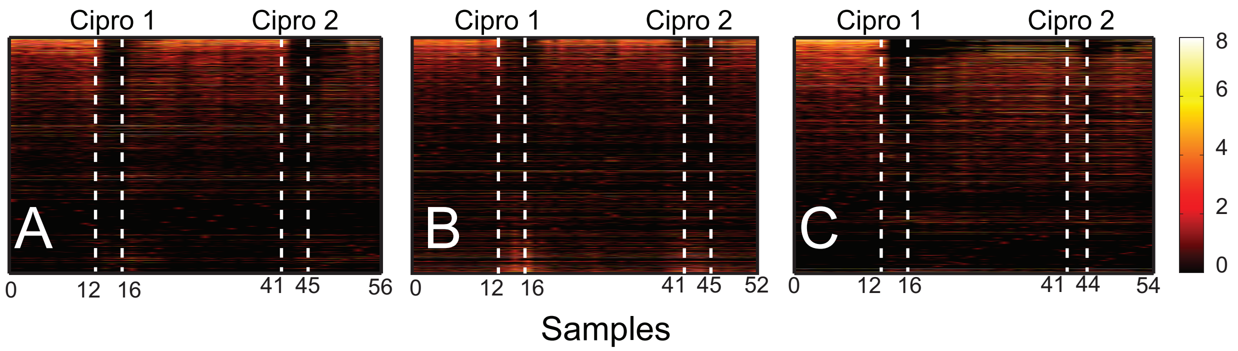


FIG. S8: *Log*$_2$ abundance versus samples for all the phylotypes detected in each individual (A, B, C) from [2] sorted from the most to least correlated with PCA1. At the top we individuate the most sensitive phylotypes to antibiotic (mostly decreasing in density) while at the bottom the most tolerant ones (mostly increasing in density). Differently from Fig. 5 in the main text, where only the top 20 sensitives and tolerants are shown, here we display all the detected phylotypes.

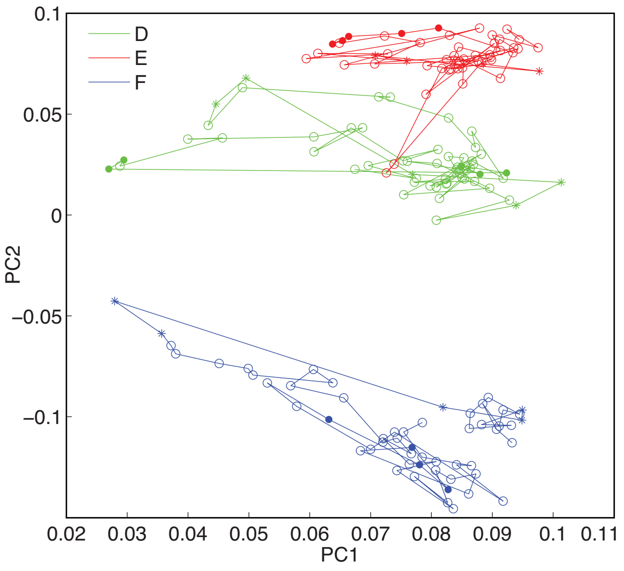


FIG. S9: Ordination plot of the time samples based on their first two principal components. We can easily recognize the time points belonging to the three individuals (inter-individual variability) and their evolution in response to treatment. Empty circles represent untreated samples, asterisks represent samples during treatment 1 and filled circles represent represent samples during treatment 2.

## IV. VIDEO S1 LEGEND

The video shows the stationary probability distributions $P_s$ as a function of the sensitive and tolerant densities for increasing noise value $D$, which ranges from $10^{-4}$ to $10^{-2}$. For visualization purposes, the noise value associated to each movie frame is displayed as an increasing bar in the top panel.

## V. VIDEO S2 LEGEND

The video shows the time evolution of the two principal components for the three subjects from [2]. Empty circles represent untreated samples, asterisks represent samples during treatement 1 and filled circles represent represent samples during treatement 2.


[1] Hsu SB, Li YS, Waltam P (2000) Competition in the presence of a lethal external inhibitor. *Math Biosc*, 167:177-199.

[2] Dethlefsen L, Relman DA (2011) Incomplete recovery and individualized responses of the human distal gut microbiota to repeated antibiotic perturbation. *Proc Natl Acad Sci U S A*, 108 Suppl 1:4554-4561.

[3] Alter O, Brown PO, Botstein D (2000) Singular value decomposition for genome-wide expression data processing and modeling. *Proc Natl Acad Sci*, 97(18):10101-10106.

[4] Otto S, Day T (2007) *A Biologist's guide to mathematical modeling* Princeton, NJ: Princeton University Press.

[5] Fay TH, Joubert SV (2010) Separatrices, *Inter. Journ. Math. Educ. Scie. Tech.* 41(3):412-419.

[6] Ubeda C et al (2010) Vancomycin-resistant enterococcus domination of intestinal microbiota is enabled by antibiotic treatment in mice and precedes bloodstream invasion in humans. *J Clin Invest*, 120(12):4332-4341.

[7] Higham DJ (2001) An algorithmic introduction to numerical simulation of stochastic differential equations. *SIAM Rev.*, 43:525-546.

[8] Gardiner CW (1983) The escape time in nonpotential systems. *J. Stat. Phys.*, 30(1):157-177.

[9] Borgis D, Moreau M (1990) On the escape rate from a metastable state in a non-potential system. *Physica A* 163:877-894.

[10] Gardiner CW (1997) Handbook of stochastic methods, Third Edition, eds Springer series in Synergetics (Spinger Hedeilberg).

[11] Mao-Jones J, Ritchie KB, Jones LE, Ellner SP (2009) How microbial community development composition regulates coral disease development. *Plos Bio.*,8(3):e1000345. doi:10.1371/journal.pbio.1000345

[12] Seifert U (2008) Stochastic thermodynamics: principles and perspectives.*EPJ B*, 64(3-4):423-431.
[13] Langer JS (1967) Theory of condensation point. *Ann Phys* 41:108-157
[14] Langer JS (1968) Theory of nucleation rates. *Phys Rev Lett*, 21(14):973-976.
[15] Sidney Coleman (1988) Aspects of symmetry, eds Cambridge University Press.
